# Supplementary material for: A classification scheme for chimera states
Source: arXiv:1603.01110 source file (2016-07-18)
Supplement: Supplementary file 1 [file suppl.pdf]

# Supplementary information to "A classification scheme for chimera states"

Felix P. Kemeth,[1,2] Sindre W. Haugland,[1,2] Lennart Schmidt,[1] Ioannis G. Kevrekidis,[2,3] and Katharina Krischer[1,a)]

[1)] *Physik-Department, Nonequilibrium Chemical Physics, Technische Universität München, James-Franck-Str. 1, D-85748 Garching, Germany*

[2)] *Institute for Advanced Study - Technische Universität München, Lichtenbergstr. 2a, D-85748 Garching, Germany*

[3)] *The Department of Chemical and Biological Engineering - Princeton University, Princeton, NJ 08544, USA*

(Dated: 15 July 2016)

## I. KURAMOTO MODEL, FIGURE 1, 2, 4 AND 5

The evolution of the phases in the Kuramoto model[1] is described by

$$\partial_t \theta(x,t) = \omega - \int G(x-x') \sin(\theta(x,t) - \theta(x',t) + \alpha)\, dx' \tag{1}$$

with the coupling kernel

$$G(x-x') = \frac{\kappa}{2} e^{-\kappa|x-x'|}. \tag{2}$$

We numerically integrate the Kuramoto model, equation (1), using the fourth-order Runge-Kutta method with fixed time step $dt = 0.025$. As initial conditions, random numbers $\sigma$ with a Gaussian envelope

$$\theta(x, t=0) = 6.0 e^{-30.0(x-L/2)^2} \cdot \sigma(x) \tag{3}$$

are taken. Further parameters are $\alpha = 1.457$, $\kappa = 4.0$, $L = 1$. As boundary conditions periodic conditions are chosen.

## II. TWO-GROUP APPROXIMATION BY ABRAMS ET AL., FIGURE 3

The dynamics in the two-group approximation by Abrams et al.[2] follow

$$\frac{d\theta_i^\sigma}{dt} = \omega + \sum_{\sigma'=1}^{2} \frac{K_{\sigma\sigma'}}{N_{\sigma'}} \sum_{j=1}^{N_{\sigma'}} \sin\left(\theta_j^{\sigma'} - \theta_i^\sigma - \alpha\right) \tag{4}$$

with the two groups $\sigma \in \{1,2\}$ and the number of oscillators in each group $N_\sigma$, which are set to $N_1 = N_2 = 512$. The coupling-strengths $K_{\sigma\sigma'}$ are taken as $K_{11} = K_{22} = 0.675$ and $K_{12} = K_{21} = 0.325$. The phase lag $\alpha = \pi/2 - 0.1$ and the frequencies $\omega = 0$ are identical for all oscillators. Initial conditions are random phases with small variance ($< 0.1$) for group one and large variance ($= 2.0$) in group two. The system is integrated using a fourth-order Runge-Kutta method with a fixed time step of $dt = 0.01$.

a)krischer@tum.de

## III. AMPLITUDE-MEDIATED CHIMERAS BY SETHIA ET AL., FIGURE 6

Sethia et al.[3] observed chimera states in the one-dimensional, nonlocal complex Ginzburg-Landau equation,

$$\frac{\partial W}{\partial t} = W - (1 + ic_2)|W|^2 W + K(1 + ic_1)\left(\bar{W} - W\right), \tag{5}$$

with $c_1 = 0.5$, $c_2 = 2.0$, $K = 0.4$, $N = 2001$ and the spatial extension $-1 \leq x \leq 1$. The coupling $\bar{W}$ is chosen as

$$\bar{W}(x,t) = \int_{-1}^{1} G(x-x') W(x-x',t) dx' \tag{6}$$

with

$$G(x) = \frac{\kappa}{2(1-e^{-\kappa})} e^{-\kappa|x|} \tag{7}$$

and $\kappa = 2$. As boundary conditions periodic boundaries are taken, and the initial conditions were taken similar to equation (3) with amplitude $A = 1$. As integrator, fourth-order Runge-Kutta with a fized time-step of $dt = 0.01$ is used.

## IV. CHIMERA STATES OBSERVED BY OMELCHENKO ET AL., FIGURE 7

Omelchenko et al.[4] used a lattice of local maps

$$\phi^{n+1} = 2\pi a I(\phi^n) \tag{8}$$

with $I(\phi) = (1 - \cos(\phi))/2$. The maps are coupled nonlocally, resulting in the underlying equation for $\phi$ on site $i$,

$$\phi_i^{n+1} = 2\pi a \left\{ I(\phi_1^n) + \frac{\epsilon}{2R} \sum_{j=-R}^{R} \left[ I(\phi_{i+j}^n) - I(\phi_i^n) \right] \right\}. \tag{9}$$

Parameters are chosen as $N = 1024$, $a = 0.85$, $\epsilon = 0.4$ and $R = 420$.

## V. COMPLEX GINZBURG-LANDAU EQUATION, FIGURE 10

The complex Ginzburg-Landau equation (CGLE),

$$\partial_t W = W + (1 + ic_1)\nabla^2 W - (1 + ic_2)|W|^2 W, \quad (10)$$

is integrated using a pseudo-spectral integration method with exponential time-stepping[5] and fixed time step $dt = 0.01$, system size $L = 1000$ and $N = 2048$. Other parameters for spatio-temporal intermittency[6] are $c_1 = 0$ and $c_2 = -3$.

## VI. COMPLEX GINZBURG-LANDAU EQUATION WITH LINEAR GLOBAL COUPLING, FIGURE 9, 11 AND 12

The CGLE with linear global coupling is given by

$$\partial_t W = W + (1 + ic_1)\nabla^2 W - (1 + ic_2)|W|^2 W \quad (11)$$
$$+\mu(1 + ic_3)(\langle W\rangle - W),$$

with $\langle\cdot\rangle$ denoting the spatial mean and $\mu$ the coupling strength. For $c_1 = 2$, $c_2 = -1.2$, $c_3 = 0$ and $\mu = 0.3$, this system shows localized turbulence patterns, and for $c_1 = 1.2$, $c_2 = 1.7$, $c_3 = -1.25$ and $\mu = 0.67$, a type I chimera can be observed. For two-dimensional simulations the CGLE with linear global coupling is integrated on a two-dimensional grid with $N \times N = 256 \times 256$ points using a pseudo-spectral integration method with exponential time-stepping[5] and fixed time step $dt = 0.01$. If not stated otherwise, the system length is taken as $L = 200$. For simulations with one spatial dimension, $L = 200$ and $N = 2048$. The initial conditions are complex random numbers with small variance ($< 0.1$) centered around the origin[7].

## VII. COMPLEX GINZBURG-LANDAU EQUATION WITH NON-LINEAR GLOBAL COUPLING, FIGURE 8

The CGLE with non-linear global coupling is described by

$$\partial_t W = -i\nu W + (1 + ic_1)\nabla^2 W - (1 + i\nu)(\langle W\rangle - W) \quad (12)$$
$$+ (1 + ic_2)\left(\langle |W|^2 W\rangle - |W|^2 W\right)$$

and has the property that for the uniform mode,

$$\partial_t\langle W\rangle = -i\nu\langle W\rangle \rightarrow \langle W\rangle = \eta e^{-i\nu t} \quad (13)$$

holds. Thus, the mean $\langle W\rangle$ is confined on a circle with frequency $\nu$ and amplitude $\eta$[8]. This system shows type II chimeras for $c_1 = 0.2$, $c_2 = -0.63$, $\nu = 0.1$ and $\eta = 0.65$, with random initial conditions. As system size $L = 1000$ and $N = 4096$ grid points are taken. For integration a pseudo-spectral method with exponential time-stepping[5] and fixed time step of $dt = 0.01$ was used.

## VIII. AMPLITUDE CHIMERA STATES OBSERVED BY ZAKHAROVA ET AL., FIGURE 13

The amplitude chimera states are found in a system of nonlocally coupled Stuart-Landau oscillators[9],

$$\dot{z}_j = \left(\lambda + i\omega - |z|^2\right) z + \frac{\sigma}{2P}\sum_{k=j-P}^{j+P}\left(\mathrm{Re}z_k - \mathrm{Re}z_j\right), \quad (14)$$

with $j = 1, 2, \ldots, N$, $z \in \mathbb{C}$, $\lambda = 1$, $\omega = 2$, $\sigma = 40$, $P = 60$ and $N = 3000$. Special care has to be taken while choosing the initial conditions, which is explained in more detail by Loos et al.[10] For integration, an implicit Adams method with a fixed time step of $dt = 0.002$ is used.

## IX. CO-OXIDATION MODEL WITH GLOBAL COUPLING, FIGURE 14

For the CO-oxidation model, the dynamics of the coverage of carbon monoxide, $c$, is modeled by

$$\partial_t c = D\nabla^2 c + k_1 p_{\mathrm{co}} s_{\mathrm{c}}\left(1 - \left(\frac{c}{c_{\mathrm{s}}}\right)^3\right) - k_2 c - k_3 co \quad (15)$$

with the diffusion coefficient for CO, $D$, the rate of CO hitting the surface, $k_1$, the partial pressure of CO, $p_{\mathrm{co}}$, the sticking coefficient of CO, $s_{\mathrm{c}}$, the saturation coverage $c_{\mathrm{s}}$, the CO-desorption rate $k_2$, the reaction rate $k_3$ and the oxygen coverage $o$. Unlike earlier studies, we assume that the diffusion process is isotropic and take the diffusion coefficient $D$ as constant. The coverage $o$ follows

$$\partial_t o = k_4 p_{\mathrm{o}_2}\left(\left(s_{\mathrm{o}_1} - s_{\mathrm{o}_2}\right) w + s_{\mathrm{o}_2}\right)\left(1 - \frac{c}{c_{\mathrm{s}}} - \frac{o}{o_{\mathrm{s}}}\right)^2 - k_3 co, \quad (16)$$

where $k_4$ is the rate of the oxygen molecules hitting the surface, $p_{\mathrm{o}_2}$ the partial pressure of these molecules in the gas phase, $s_{\mathrm{o}_1}$ and $s_{\mathrm{o}_2}$ are the sticking coefficients of oxygen on the $1 \times 1$ and $1 \times 2$ surface structure, respectively, and $o_{\mathrm{s}}$ is the saturation coverage of $o$. Notice that the adsorption of oxygen depends on the surface structure, $w$. This variable can be described by

$$\partial_t w = k_5\left(g\left(\frac{c}{c_{\mathrm{s}}}\right) - w\right) \quad (17)$$

with the function $g(x)$,

$$g(x) = \begin{cases} 0 & \text{if } 0 \le x < 0.2 \\ -\frac{x^3 - 1.05x^2 + 0.3x - 0.026}{0.0135} & \text{if } 0.2 \le x \le 0.5 \\ 1 & \text{if } 0.5 < x \le 1.0. \end{cases} \quad (18)$$

Falcke and Engel introduced a global coupling through the gas phase through the partial pressure $p_{\mathrm{co}}$[11]. The equation for changes of $p_{\mathrm{co}}$, equation (19), results from a

| | | |
|---|---|---|
| Rate of CO hitting the surface | $k_1$ | $4.18 \cdot 10^5\,\mathrm{s}^{-1}\mathrm{Torr}^{-1}$ |
| CO sticking coefficient | $s_\mathrm{c}$ | 1 |
| CO saturation coverage | $c_\mathrm{s}$ | 1 |
| Rate of $O_2$ hitting the surface | $k_4$ | $4.18 \cdot 10^5\,\mathrm{s}^{-1}\mathrm{Torr}^{-1}$ |
| $O_2$ sticking coefficient on $1 \times 1$ | $s_{\mathrm{o}_1}$ | 0.6 |
| $O_2$ sticking coefficient on $1 \times 2$ | $s_{\mathrm{o}_2}$ | 0.4 |
| $O_2$ saturation coverage | $o_\mathrm{s}$ | 0.8 |
| Reaction rate | $k_3$ | $A_3 = 3 \cdot 10^6\,\mathrm{s}^{-1}$ , $E_3 = 10\,\mathrm{kcal/mol}$ |
| CO desorption rate | $k_2$ | $A_2 = 2 \cdot 10^{16}\,\mathrm{s}^{-1}$ , $E_2 = 38\,\mathrm{kcal/mol}$ |
| Surface structure transition rate | $k_5$ | $A_5 = 10^2\,\mathrm{s}^{-1}$ , $E_5 = 7\,\mathrm{kcal/mol}$ |
| Diffusion coefficient | D | $10 \cdot 10^{-12}\,\mathrm{m}^2/\mathrm{s}$ |
| Temperature | T | 545 K |
| Partial pressure of CO in the gas inflow | $p_\mathrm{coe}$ | $3.992 \cdot 10^{-5}$ Torr |
| Reactor volume | $V$ | 50 l |
| Gas flow into the reactor | $J$ | 360 l/s |
| Partial pressure of $O_2$ | $p_{\mathrm{o}_2}$ | $1.17 \cdot 10^{-4}$ Torr |
| Volume of a mono-layer | $V_\mathrm{ML}$ | 0.3 l/ML |
| Length of the electrode | $L$ | $L = 1800\,\mu\mathrm{m}$ |

TABLE I. Parameters for the CO-oxidation model (15) to (19)

$$\partial_t p_\mathrm{co} = \frac{J}{V}\left(p_\mathrm{coe} - p_\mathrm{co}\left(1 + \frac{V_\mathrm{ML}}{JL}\int\left[k_1 p_\mathrm{co}\left(1 - \left(\frac{c}{c_\mathrm{s}}\right)^3\right) - k_2\frac{c}{c_\mathrm{s}}\right]dr\right)\right) \tag{19}$$

constant inflow with $p_\mathrm{coe}$, outflow with $p_\mathrm{co}$ and changes through adsorption and desorption. This can be summarized as shown in equation (19), with $J$ denoting the gas flow into the reactor, $A$ the surface area, $V$ the reactor volume and $V_\mathrm{ML}$ the volume of a mono-layer[11]. The parameters for this model are summarized in table I[11,12]. Hereby the reaction rates $k_i$ for $i = 2, 3, 5$ follow the Arrhenius equation

$$k_i = A_i e^{-E_i/(RT)}. \tag{20}$$

Integration parameters are $N = 3600$ and $L = 1800\,\mu\mathrm{m}$, and a fourth-order Runge-Kutta method with fixed time step $dt = 10^{-4}$ s is used.


[1] Y. Kuramoto and D. Battogtokh, "Coexistence of coherence and incoherence in nonlocally coupled phase oscillators," Nonlinear Phenom. Complex Syst. **5**, 380–385 (2002).

[2] D. M. Abrams, R. Mirollo, S. H. Strogatz, and D. A. Wiley, "Solvable model for chimera states of coupled oscillators," Phys. Rev. Lett. **101**, 084103 (2008).

[3] G. C. Sethia, A. Sen, and G. L. Johnston, "Amplitude-mediated chimera states," Phys. Rev. E **88**, 042917 (2013).

[4] I. Omelchenko, Y. Maistrenko, P. Hövel, and E. Schöll, "Loss of Coherence in Dynamical Networks: Spatial Chaos and Chimera States," Physical Review Letters **106**, 234102 (2011).

[5] S. Cox and P. Matthews, "Exponential Time Differencing for Stiff Systems," Journal of Computational Physics **176**, 430–455 (2002).

[6] B. Shraiman, A. Pumir, W. van Saarloos, P. Hohenberg, H. Chat, and M. Holen, "Spatiotemporal chaos in the one-dimensional complex Ginzburg-Landau equation," Physica D: Nonlinear Phenomena **57**, 241 – 248 (1992).

[7] D. Battogtokh, A. Preusser, and A. Mikhailov, "Controlling turbulence in the complex Ginzburg-Landau equation II. Two-dimensional systems," Physica D: Nonlinear Phenomena **106**, 327–362 (1997).

[8] L. Schmidt, K. Schönleber, K. Krischer, and V. García-Morales, "Coexistence of synchrony and incoherence in oscillatory media under nonlinear global coupling," Chaos **24**, 013102 (2014).

[9] A. Zakharova, M. Kapeller, and E. Schöll, "Chimera death: symmetry breaking in dynamical networks," Phys. Rev. Lett. **112**, 154101 (2014).

[10] S. A. M. Loos, J. C. Claussen, E. Schöll, and A. Zakharova, "Chimera patterns under the impact of noise," Phys. Rev. E **93**, 012209 (2016).

[11] M. Falcke and H. Engel, "Influence of global coupling through the gas phase on the dynamics of CO oxidation on Pt(110)," Phys. Rev. E **50**, 1353–1359 (1994).

[12] K. Krischer, M. Eiswirth, and G. Ertl, "Oscillatory CO oxidation on Pt(110): Modeling of temporal self-organization," The Journal of Chemical Physics **96**, 9161–9172 (1992).
